# Supplementary material for: Mixed approximation of nonlinear acoustic equations: Well-posedness and a priori error analysis
Source: arXiv:2209.02737 source file (2022-09-06)
Supplement: Supplementary file 1 [file appendix.tex]

\begin{appendices}
\section{On the pressure-velocity formulation of acoustic equations} \label{SubSec:PressureVelocity}
In ultrasound applications, one might also be interested in directly computing the acoustic pressure instead of the potential. We point to~\cite[Chapter 5]{kaltenbacher2007numerical} for links between pressure and potential formulations of acoustic equations. We discuss in this appendix how the framework of our previous analysis extends to the pressure-velocity formulation of the damped Kuznetsov equation. For an analogous comparison in the setting of linear elastodynamics, we refer to \cite{makridakis1992mixed}.

Having already introduced the velocity in \eqref{eq:continuous_mixed_problem}, we note that the pressure is given by $u=-\varrho \psi_t$.  Without loss of generality, we set $\varrho=1$.  Then the Kuznetsov equation in pressure-velocity form becomes a first-order problem in time:
\begin{equation}\label{eq:continuous_mixed_problem_pressurev}
	\left \{ \begin{aligned}
		&(1-2ku)u_{t}+c^2 \nabla \cdot \bv +b \, \nabla \cdot \bvt - 2\sigma  \boldsymbol{v} \cdot \boldsymbol{v}_t=f,\\[2mm]
		& \boldsymbol{v}_t= - \nabla u.
	\end{aligned}\right.
\end{equation}
The system is coupled with boundary and initial conditions:
\begin{align}
	& u|_{\partial\Omega} = 0 , \quad  u(0)=-\psi_1, \quad \bv(0)=\nabla \psi_0.
\end{align}
The semi-discrete weak form of the pressure-velocity formulation is thus
\begin{equation} \label{IBVP_approx_Kuznetsov_pressurev}
	\left \{\begin{aligned}
		& \begin{multlined}[t]((1-2k u_{h})u_{ht}, \phi_h)_{L^2}+ c^2 (\nabla \cdot (\bvh+\tfrac{b}{c^2}\bvht), \phi_h)_{L^2}\\-2 \sigma(\boldsymbol{v}_h \cdot \bvht, \phi_h)_{L^2}= (f, \phi_h)_{L^2}, \end{multlined}\\[2mm]
		& (\bv_{ht}, \boldsymbol{w}_h)_{L^2}-(u_h, \nabla \cdot \boldsymbol{w}_h)_{L^2}=0,
	\end{aligned} \right.
\end{equation} 
for all $(\phi_h, \bwh) \in \spaceS \times \spaceV$ a.e.\ in time, with approximate initial conditions
\begin{equation}\label{eq:pressurev_init}
	\begin{aligned}
		(\ \_ \ , \bv_{0h})=(\tildePp{\psi_0}, \tildePv{\bv_0}), \\
		(u_{0h}, \bv_{1h})=(\tildePp{\psi_1}, \tildePv{\bv_1}).
	\end{aligned} 
\end{equation}
Here $\psi_0$, $\bv_1$ are obtained through
\begin{align}
	\prodLtwo{\bv_i}{\bw} + \prodLtwo{\psi_i}{\div \bw} = 0,
\end{align}
where for $i = 0$ the known is $\bv_0$ and for $i=1$, the known is $\psi_1$.
The energy and error analysis is now based on the following total pressure-velocity energy:
\begin{equation}
	\begin{aligned}
		\mathcal{E}[u, \bv](t)=E_{u}(t)+E_{\bv}(t), \ t \geq 0,
	\end{aligned}
\end{equation}
obtained by adding
\begin{equation}
	\begin{aligned}
		E_{u}(t)=\nLtwo{u(t)}^2+\int_0^t\nLtwo{u_t(s)}^2\ds
	\end{aligned}
\end{equation}
to the velocity energy $E_{{\bv}}=E_{{\bv}}(t)$, defined in \eqref{eq:kinetic_energy}.

With the next result, we extend the previous analysis framework to the pressure-velocity form.
\begin{proposition} \label{Thm:pressurev} Let $b>0$. Let $2 \leq r \leq p^*$, and 
	let $\psi \in X_{r+1}$ denote the weak solution of the exact problem with a sufficiently smooth source term $f$, and coupled with homogeneous Dirichlet data and suitable initial conditions $(\psi(0),\psi_t(0))=(\psi_0,\psi_1)$ and let $v = \nabla \psi$, $u =  - \psi_t$.  Let the approximate initial data be chosen as in \eqref{eq:pressurev_init}.
	Then there exists $\overline{h} = \overline{h}(\|\psi\|_{X_{r+1}})<1$ and $M=M(k, \sigma, T)>0$, such that for $0<h<\overline h$
	and 
	\begin{equation}
		\sup_{t \in (0,T)}\|\bv(t)\|^2_{L^{\infty}}+\sup_{t \in (0,T)}\|u(t)\|^2_{L^\infty} +\int_0^T \left( \|u_t(s)\|_{L^\infty}^2 + \|\bvt(s)\|^2_{L^\infty} \right)\ds \leq M,	\end{equation}
	there is a unique $(u_h, \bv_h)$ in the ball
	\begin{equation}
		\begin{aligned}
			\mathcal{B}_u=\left\{\vphantom{\int_0^t}\right. &(u_h^*, \bv^*_h) \in H^1(0,T; \spaceS) \times C^{1}([0,T]; \spaceV):\, \\ &\sup_{t \in (0,T)}\mathcal{E}[u-u^*_h, \bv-\bvh^*](t) \leq C_*^2 h^{2r} \|\psi\|^2_{X_{r+1}},\ \,
			(u^*_h, \bv^*_h)\vert_{t=0}=(u_{0h}, \bv_{0h})\left.\vphantom{\int_0^t}\right\},
		\end{aligned}
	\end{equation}
	with $C_*$ depending on final time $T$ and M, which solves \eqref{IBVP_approx_Kuznetsov_pressurev}. 
	\begin{comment}	\color{green}
		Furthermore, the approximate acoustic pressure satisfies	
	\begin{equation}
		\begin{aligned}
			\|\psi_t(t)-u_h(t)\|_{L^\infty} \lesssim&\, \begin{multlined}[t]  h^r \log \frac{1}{h} \|\psi\|_{X_{r+1}}\  \ \textrm{for all} \ t \in [0,T].
			\end{multlined}
		\end{aligned}
	\end{equation}
\color{black}
	\end{comment}
\end{proposition}
\begin{proof}
	The proof follows along the lines of Proposition~\ref{Prop:LinStability} and Theorem~\ref{Thm:Kuzn}. We highlight here the main differences.  \\
	\indent Studying a linearized problem of \eqref{IBVP_approx_Kuznetsov_pressurev}, one establishes similar stability bounds to those obtained in Proposition~\ref{Prop:LinStability} using the following testing strategy : \[\textup{I}\cdot(u_h+\gamma u_{ht})+(\textup{II}+\gamma\textup{II}_{t})\cdot c^2 (\bvh+\tfrac{b}{c^2}\bvht),\]
	with $\gamma = \tfrac{b}{c^2}$, where I and II represent the first and second equation in the linearization of \eqref{IBVP_approx_Kuznetsov_pressurev}, respectively. Adapting Assumption~\ref{Assumption_reg} (changing $\psi_{ht}$ to $u_h$), one retrieves a linear error estimate.
	The well-posendess and convergence of the nonlinear pressure-velocity approximation of the Kuznetsov equation follows by a fixed-point argument in the ball $\mathcal{B}_u$. The rest of the arguments follow analogously. We omit the details here.
\end{proof}
%\color{green}
\begin{remark}
	Starting from the pressure velocity-formulation and given the relationship $u = -\psi_t$ (and $u_h = -\psi_{ht}$), one can recover the bound $\|\psi_{ht}(t) - \psi_t(t)\|_{L^q}$ with the assumptions on $q$ as in Lemma~\ref{lem:elliptic_bounds} provided we have 
	\begin{align}
		\prodLtwo{\bv_{0h}}{\bw} + \prodLtwo{\psi_{0h}}{\div \bw} = 0,
	\end{align}
	and use Lemma~\ref{lem:elliptic_bounds}. 
\end{remark}
\color{black}
\end{appendices}
